# Supplementary material for: Sibling Regression for Generalized Linear Models
Source: arXiv:2107.01338 source file (2021-07-07)
Supplement: Supplementary file 1 [file appendix.tex]

\appendix
\onecolumn

\section{Proof of Proposition \ref{claim:reg}}
\label{apx:proof_reg}

\begin{proof} First we write $\Rs(Y_i) = Z_i + N - X^T\hat{\beta}_i + \eps_i$ where $\eps_i$ is a random error term. For notational convenience we supress the dependence of $\eps_i$ $Z,N,X$.
Given $X$, randomness in $\Rs(Y_i)$ is a purely due to randomness in $Y_i$.  From the causal diagram \ref{fig:sglm-sibling} we can see that $Y_i \indep X,Y_{-i} |Z_i,N$. This implies that $\eps_i \indep X,Y_{-i} |Z_i,N$. \\
\iffalse{
Since $\E [\Rs(Y_i)| X, N] = Z_i + N - X^T\hat{\beta}_i$, we get, $\E[eps_i| X, N] = 0$
\begin{align*}
&\E [\Rs(Y_i)| X, N] - (Z_i + N - X^T\hat{\beta}_i)  = 0\\ 
\E [Z_i + N - X^T\hat{\beta}_i + \eps_i| X, N] =  Z_i + N - X^T\hat{\beta}_i \\
\E [Z_i|X] + N - X^T\hat{\beta}_i + \E[eps_i| X, N] =  Z_i + N - X^T\hat{\beta}_i \\
\E[eps_i| X, N] = Z_i - \E [Z_i|X]
\end{align*}
}\fi
Note from the assumption that $ Z_i + N - X^T\hat{\beta}_i$ is the true expectation. Since $\eps_i$ is deviation from the true expectation :
$\forall Z_i,N: \E[\eps_i | Z_i,N] = 0 $
\begin{align*}
    \E[\eps_1|Y_2,X] &= \E[\E[\eps_1|Z_1,N,Y_2,X]|X,Y_2] = \E[\E[\eps_1|Z_1,N]|X,Y_2] = \E[0|X,Y_2] = 0
\end{align*}
We first use law of iterated expectation to condition on $Z_1,N$. Next we use independence between $\eps$ and $X,Y_2$. Finally we set the conditional expectation to $0$.
Now using the above result we can write:
\begin{align*}
 \E [\Rs(Y_1)| X, \Rs(Y_2)] &= \E [ Z_1 + N - X^T\hat{\beta}_1 + \eps_1| X, \Rs(Y_2)] \\
 &=  \E [ N | X, \Rs(Y_2)] + \E [ Z_1 - X^T\hat{\beta}_1| X, \Rs(Y_2)] + \E[\eps_1| X, \Rs(Y_2)] \\
 &= \E [ N | X, \Rs(Y_2)] + \underbrace{
\E[Z_1|X] - X^T\hat{\beta}_1}_{f(X)} = \E [ N | X, \Rs(Y_2)] + f(X)
\end{align*}
The last equality follows from the fact that $\E[Z_1|X] - X^T\hat{\beta}_1$ is purely a function of $X$ (labeled $f(X)$ ). Similarly $ \E [\Rs(Y_1)| X] = \E [ N | X] + f(X) = f(X) $ \\
Combining the two we get:
$$ \E[\Rs(Y_1)| X, \Rs(Y_2)] - \E [\Rs(Y_1)| X] =  \E [ N | X, \Rs(Y_2)] $$
\end{proof}

\section{Experimental Results: Gamma Regression}

Figure \ref{fig:bias_appx} shows the estimation error for Gamma regression as a function of the dimension $n$ of $Y_{-1}$, i.e., the number of auxiliary variables. Figure \ref{fig:bias_appx}(a) plots the bias against the true value of $Z_1$ while Figure~\ref{fig:bias_appx}(b,c) depicts the MSE of using  different residuals and the method of \cite{3qs} 
\begin{figure}[h!]
\subfigure[]{
  \includegraphics[width=0.27\textwidth]{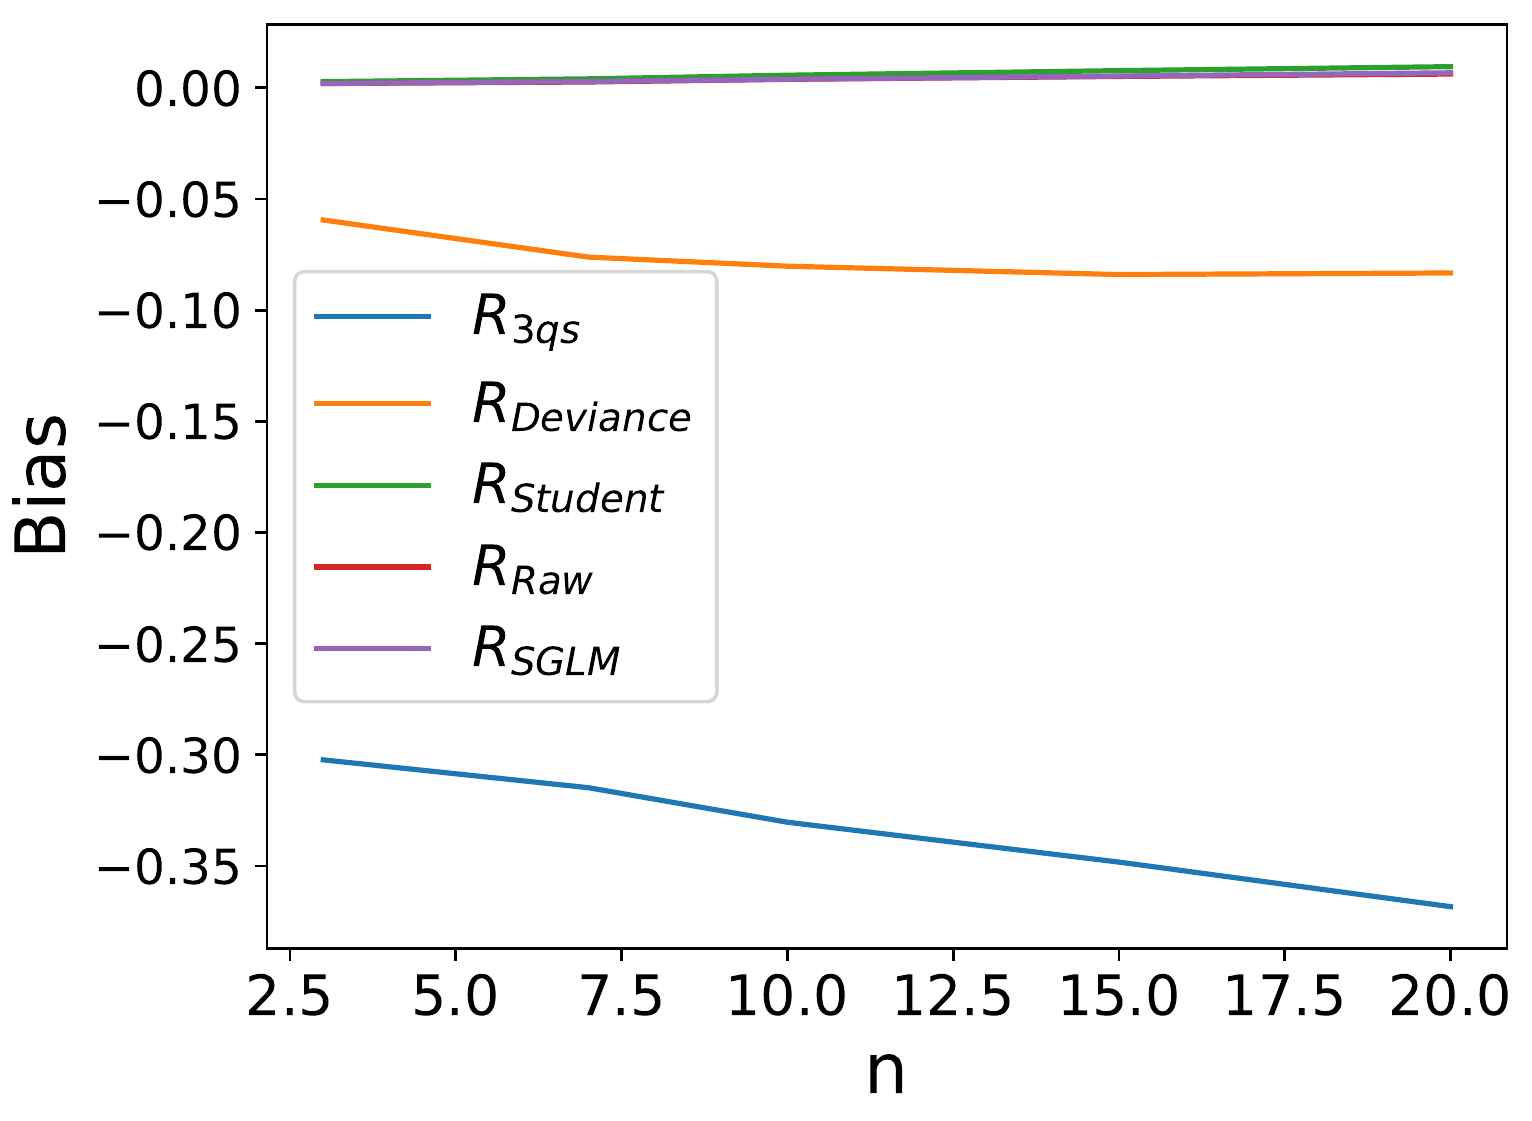}
  }
\subfigure[]{
  \includegraphics[width=0.27\textwidth]{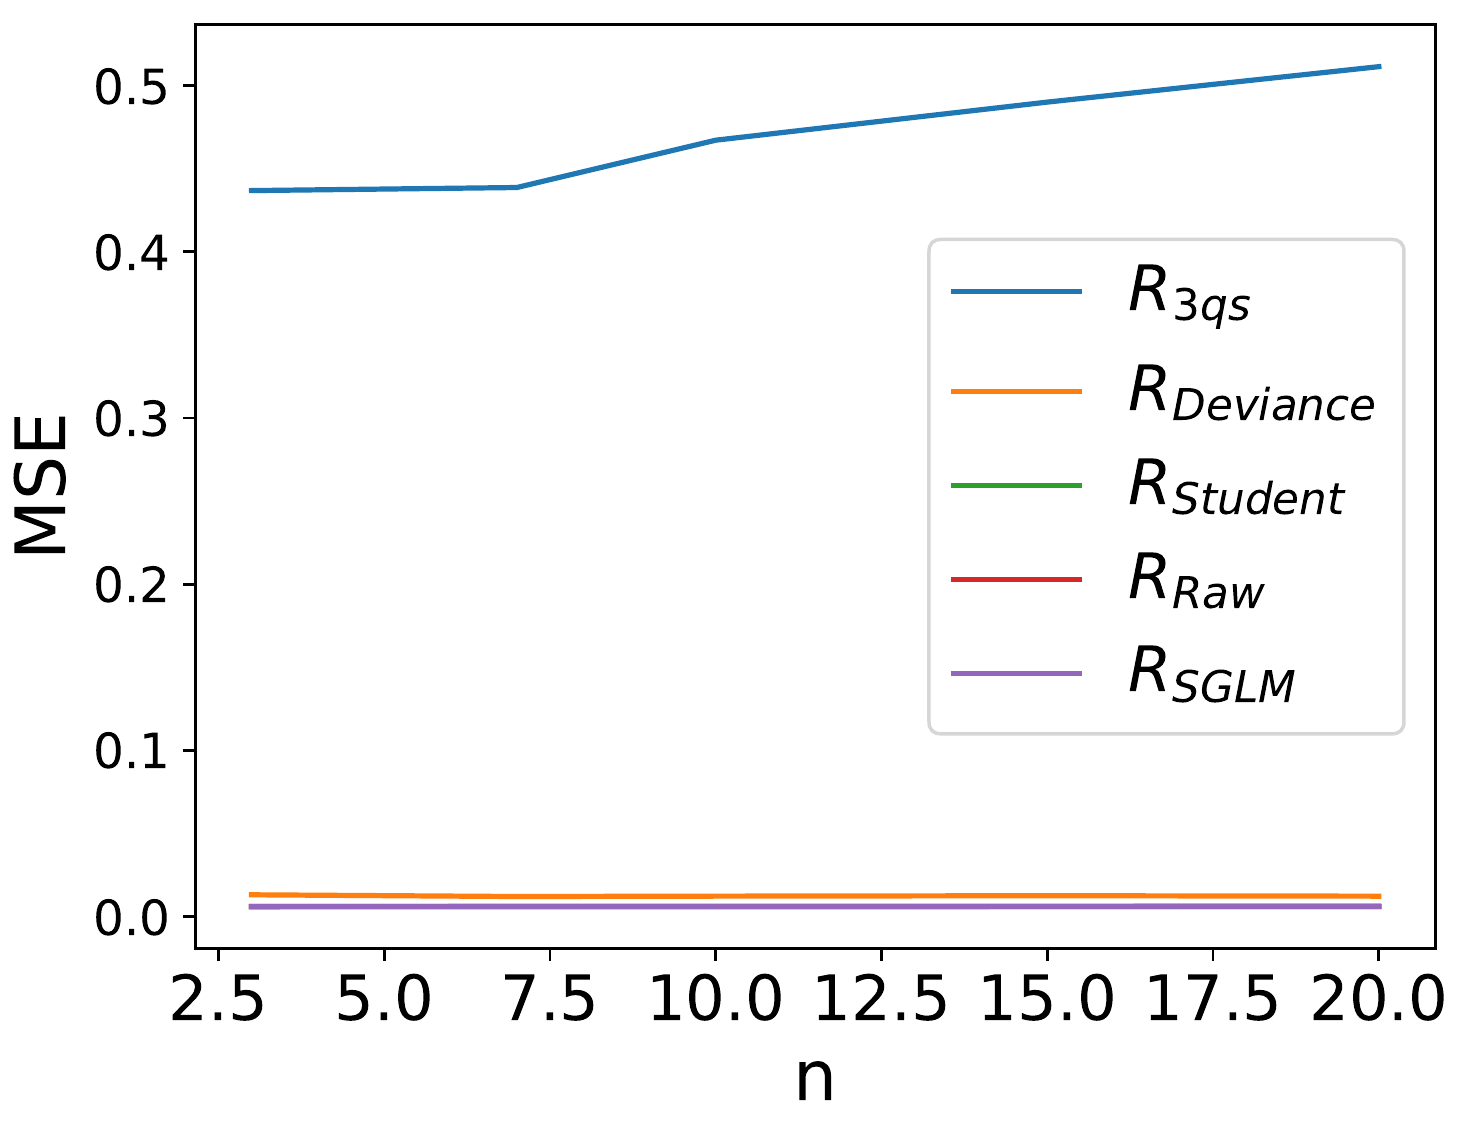}
}
\subfigure[]{
  \includegraphics[width=0.27\textwidth]{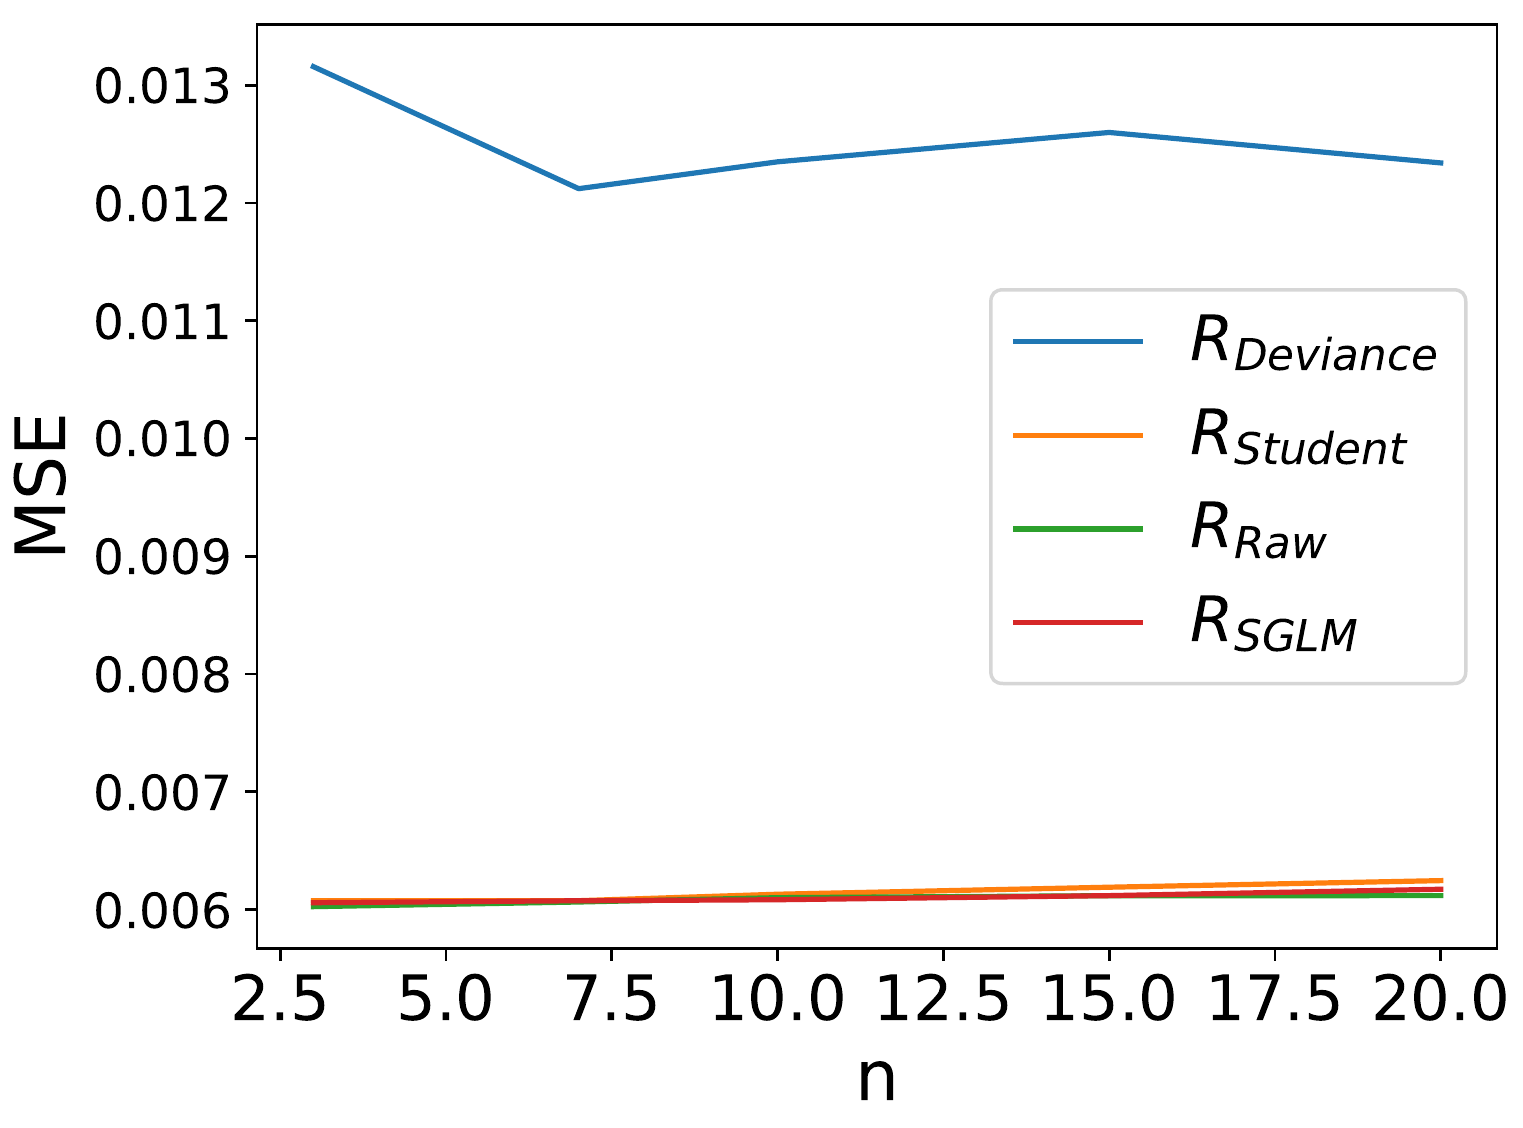}
}
  
  %\caption{Results on synthetic data. MSE and Bias vs $|Y_2|$ count $n$ for (a) Poisson regression and (b) Gamma regression \label{fig:mse}}

\caption{Results on synthetic data. Bias (a),  and MSE for various Residual comparison (b,c) vs $|Y_2|$ count $n$ on Gamma regressions \label{fig:bias_appx}}
%\end{figure*}
\end{figure}

\section{Improving estimate of $N$ using more auxiliary variables}
\label{apx:heuristic}
Let the approximation in Claim \ref{claim:resid} be exact i.e
$\E [\Rs(Y_i)| X, N] = Z_i + N - X^T\hat{\beta}_i$. Furthermore assume that $Z_i = h_i(X) + \gamma_i$ where $\gamma_i$ are 0 mean independent random variables capturing the variability of $Z_i$ not captured in $X$.\\
From the causal diagram \ref{fig:glm-sibling} one can observe that conditioned on $X,N$ all $Y_i$ are independent. This means if we restrict ourselves to the observations which share the value of $X,N$ (condition on same $X,N$), then by law of large numbers the average of $\Rs$ converges to the average of their expectations.
\begin{align*}
\lim_{k\rightarrow \infty} \dfrac{\sum_i^{k} \Rs(Y_i) }{k} &\xrightarrow[]{P} \dfrac{\sum_i^{k} \E[\Rs(Y_i)|X,N] }{k} = \dfrac{\sum_i^{k} (Z_i + N - X^T\hat{\beta}_i) }{k}\\
%&= N + \dfrac{\sum_i^{k} Z_i }{k} - X^T\dfrac{\sum_i^{k} \hat{\beta}_i}{k}\\
&= N + \dfrac{\sum_i^{k} h_i(X) + \gamma_i - X^T\hat{\beta_i}}{k} \\
%&\xrightarrow[]{P} N + \dfrac{\sum_i^{k} h_i(X) + \gamma_i}{k} - X^T\dfrac{\sum_i^{k} \hat{\beta}_i}{k}\\
&= N + \dfrac{\sum_i^{k} \gamma_i }{k} + r(X)\\
&\xrightarrow[]{P} N + \dfrac{\sum_i^{k} \E[\gamma_i] }{k} + r(X)\\
&= N + r(X)
\end{align*}

where in the second-last line we have again used the law of large numbers on the average of $\gamma_i$'s.
Informally this suggests that by combining information over many $Y$'s we can get an accurate estimate of $N$.

\section{GLM Residuals}
We conducted experiments with different measures of residuals have been used in literature \cite{belsley2005regression}. Here we provide equations for them.
\begin{itemize}
    \item $R_{\text{raw}}$ = $Y - \hat{Y}$ are the raw residuals i.e the difference between the observed value and the estimate
    \item $R_{\text{student}}$ = $\frac{Y - \hat{Y}}{\sqrt{V(\hat{Y}) (1-\text{diag}(H)}}$ is the analogue of studentized residuals in ordinary linear regression scaled their variances. $H$ is the 'hat' matrix of the model.
    \item $R_{\text{deviance}}$ = $\text{sign}(Y - \hat{Y})\sqrt{D}$ where $D$ is the contribution to the model deviance from the observation. It is the (signed) difference between the log probability of the observation given by the fitted model, and the best model
    
\end{itemize}

\section{Asymptotic Efficiency}
\label{apx:proof_asymp}
To analyze the asymptotic behavior of our approach, we rely on the following result regarding maximum likelihood estimation of misspecified models \citep{white_1994} .

\begin{theorem}
Let $D_{1,2,..n}$ be $n$ observations sampled from the distribution $P_G$. Let $\hat{\beta}_n$ be the maximum likelihood estimate obtained by optimizing $ n^{-1} \sum_i log P_F(D_i, \beta)$ where $P_F(.,\beta)$ is a parametric model. Then under certain assumptions %\\
$$
\sqrt{n}(\hat{\beta}_n - \beta^*) \xrightarrow[]{a.s} \mathcal{N} (0,C(\beta^*)) \text{ as } n \rightarrow \infty
$$

where $\beta*$ is the value of parameters which minimizes the KL divergence between the true and misspecified models and $C$ is a covariance matrix functional dependent on $P_F$ and $P_G$.
\end{theorem}
In the second stage estimation (Step 5 in Algorithm \ref{alg:calibrate}) we use maximum likelihood training to re-estimate the GLM models with $\E[\Rs(Y_i)|\Rs(Y_{-i})]$ as a proxy for the noise variable. Hence the above result directly applies showing that our estimate of parameters is asymptotically normal.

To derive the relative efficiency of the SGLM approach vis a vis direct estimation, we compute the functional $C$ using the following expressions from \citet{white_1994}:
\begin{align*}
    C = \bar{A}^{-1}(\theta^*)\bar{B}(\theta^*)\bar{A}^{-1}(\theta^*) \\
    \bar{A} = \E_{P_G} [\dfrac{\partial^2 log P_F(Y|X,\theta^*)}{\partial \theta_i^* \partial \theta_j^* }] \\
    \bar{B} = \E_{P_G} [\dfrac{\partial log P_F(Y|X,\theta^*)}{\partial \theta_i^* } \dfrac{\partial log P_F(Y|X,\theta^*)}{\partial \theta_j^* }]
\end{align*}

where $\E_{P_G}$ is expectation with respect to the true distribution $P_G$.

Let the covariates available in the fitted model be denoted as $X_c$. For the standard max likelihood estimation, the covariates $X_c$ are $X$. On the other hand in SGLM we have an additional covariate obtained from the residuals. Note that for simplicity of exposition instead of explicitly writing this as an expectation like $\E[\Rs(Y_1)|\Rs(Y_2)$, we abuse notation to denote the term by $\Rs$.

Then using the definition of canonical GLMs for the generative model in Figure \ref{fig:glm-sibling} we get:
\begin{align*}
\bar{B} &= \E_{X,N} [ X_c^TX_c  \E_{Y|X,N} [ (Y - A'(\beta^* X_c))^2 ] ] \\ &= \E_{X,N} [ X_c^TX_c ( Var(Y|X,N) + (\E[Y|X,N] - A'(\beta^* X_c))^2)) ]  \\
\bar{A} &= \E_{X,N} [ X_c^TX_c \E_{Y|X,N} [ A''(\beta^* X_c)] ]
\end{align*}

%We will use Assumption
In the current generative model analysing the above expressions without further assumptions is intractable. Hence we limit to the  the test for no effect of covariate factors i.e under the null hypothesis that $Z_i$ being linearly independent of $X$. Under this hypothesis, both $\E[Y|X,N]$ and $Var[Y|X,N]$  becomes independent of covariates $X$ and hence can be treated purely as a function of $N$. Secondly since the variance explicitly depends on the optimal $\beta^*$ which again depends on the specific distribution of $N,X$, we make another assumption that the estimated $\beta^*$ are close enough to 0, to treat $\bar{A}$ as a constant matrix.

Under these assumptions, the terms including the log partition function $A$ also become independent of $X$, allowing a factorization of the above expectations into product of expectations. Specifically we can factor out the $X^TX$ terms (as $X$ is independent of $N$).
Finally we use Proposition \ref{claim:reg} to argue that $N = \Rs + \epsilon_N $ where $\epsilon_N$ is unpredictable independent error of reconstructing $N$. \\

Simple algebra then shows that for standard GLM estimation:\\
$\begin{aligned}[t] % placement: default is "center", options are "top" and "bottom"
B &= \E_N [ (Var(Y|N) + ( A'(\beta_N N) - A'(0))^2) ] \approx  \E_N [ (Var(Y|N)] + (\beta_N A''(0))^2 Var(N) ] \\
\end{aligned}$ 
\\ \textbf{}\\
On the other while for SGLM we get:\\
$\begin{aligned}[t] % placement: default is "center", options are "top" and "bottom"
B &= \E_N [ (Var(Y|N) + ( A'(\beta_N N) - A'( \beta_N \Rs))^2) ] \approx  \E_N [ (Var(Y|N)] + (\beta_N A''(0))^2 Var(\eps_N) ] \\
\end{aligned}$

From the above expressions it is clear that the asymptotic relative variance of the estimator is determined by the strength of dependence on noise $\beta_N$, the inherent variability of $Y$ and the reconstruction error of $N$ from the residuals. When the reconstruction error is small (such as when the number of auxiliary variables is high) then SGLM can provide more powerful tests and better confidence intervals for parameter estimation. Similarly as one might expect if the conditional variance of $Y$ is very high compared to the influence of $N$ both methods have similar efficiency.

%\pen ageweve habreak
