# Supplementary material for: Sibling Regression for Generalized Linear Models
Source: arXiv:2107.01338 source file (2021-07-07)
Supplement: Supplementary file 3 [file GLM_half_sibling_regression_supp.pdf]

## A Proof of Claim 3

*Proof.* First we write  $\mathcal{R}(Y_i) = Z_i + N - X^T \hat{\beta}_i + \epsilon_i$  where  $\epsilon_i$  is a random error term. While  $\epsilon_i$  can have non-trivial dependence on  $Z, N, X$ , we suppress that for notational convenience.

Given  $X$ , randomness in  $\mathcal{R}(Y_i)$  is a purely due to randomness in  $Y_i$ . From the causal diagram 2(c) we can see that  $Y_i \perp\!\!\!\perp X, Y_{-i} | Z_i, N$ . This implies that  $\epsilon_i \perp\!\!\!\perp X, Y_{-i} | Z_i, N$ .

Note from the assumption that  $Z_i + N - X^T \hat{\beta}_i$  is the true expectation. Since  $\epsilon_i$  is deviation from the true expectation :  $\forall Z_i, N : \mathbb{E}[\epsilon_i | Z_i, N] = 0$

$$\mathbb{E}[\epsilon_1 | Y_2, X] = \mathbb{E}[\mathbb{E}[\epsilon_1 | Z_1, N, Y_2, X] | X, Y_2] = \mathbb{E}[\mathbb{E}[\epsilon_1 | Z_1, N] | X, Y_2] = \mathbb{E}[0 | X, Y_2] = 0$$

We first rewrite the expectation to condition on  $Z_1, N$  via the law of iterated expectation. Next we use the independence between  $\epsilon$  and  $X, Y_2$ . Finally we set the conditional expectation to 0. Now using the above result we can write:

$$\begin{aligned} \mathbb{E}[\mathcal{R}(Y_1) | X, \mathcal{R}(Y_2)] &= \mathbb{E}[Z_1 + N - X^T \hat{\beta}_1 + \epsilon_1 | X, \mathcal{R}(Y_2)] \\ &= \mathbb{E}[N | X, \mathcal{R}(Y_2)] + \mathbb{E}[Z_1 - X^T \hat{\beta}_1 | X, \mathcal{R}(Y_2)] + \mathbb{E}[\epsilon_1 | X, \mathcal{R}(Y_2)] \\ &= \mathbb{E}[N | X, \mathcal{R}(Y_2)] + \underbrace{\mathbb{E}[Z_1 | X] - X^T \hat{\beta}_1}_{f(X)} = \mathbb{E}[N | X, \mathcal{R}(Y_2)] + f(X) \end{aligned}$$

The last equality follows from the fact that  $\mathbb{E}[Z_1 | X] - X^T \hat{\beta}_1$  is purely a function of  $X$  which we label as  $f(X)$ . Similarly  $\mathbb{E}[\mathcal{R}(Y_1) | X] = \mathbb{E}[N | X] + f(X) = f(X)$

Combining the two we get:

$$\mathbb{E}[\mathcal{R}(Y_1) | X, \mathcal{R}(Y_2)] - \mathbb{E}[\mathcal{R}(Y_1) | X] = \mathbb{E}[N | X, \mathcal{R}(Y_2)]$$

□

## B Improving estimate of $N$ using more auxiliary variables

Let the approximation in Claim 2 be exact i.e  $\mathbb{E}[\mathcal{R}(Y_i) | X, N] = Z_i + N - X^T \hat{\beta}_i$ . Furthermore assume that  $Z_i = h_i(X) + \gamma_i$  where  $\gamma_i$  are 0 mean independent random variables capturing the variability of  $Z_i$  not captured in  $X$ .

From the causal diagram 2(c) one can observe that conditioned on  $X, N$  all  $Y_i$  are independent. This means if we restrict ourselves to the observations which share the value of  $X, N$  (condition on same  $X, N$ ), then by law of large numbers the average of  $\mathcal{R}$  converges to the average of their expectations.

$$\begin{aligned} \lim_{k \rightarrow \infty} \frac{\sum_i^k \mathcal{R}(Y_i)}{k} &\xrightarrow{P} \frac{\sum_i^k \mathbb{E}[\mathcal{R}(Y_i) | X, N]}{k} = \frac{\sum_i^k (Z_i + N - X^T \hat{\beta}_i)}{k} \\ &= N + \frac{\sum_i^k h_i(X) + \gamma_i - X^T \hat{\beta}_i}{k} \\ &= N + \frac{\sum_i^k \gamma_i}{k} + r(X) \\ &\xrightarrow{P} N + \frac{\sum_i^k \mathbb{E}[\gamma_i]}{k} + r(X) \\ &= N + r(X) \end{aligned}$$

where in the second-last line we have again used the law of large numbers on the average of  $\gamma_i$ 's. Informally this suggests that by combining information over many  $Y$ 's we can get an accurate estimate of  $N$ .

## C Asymptotic Efficiency

To analyze the asymptotic behavior of our approach, we rely on the following result regarding maximum likelihood estimation of misspecified models (White, 1994).

**Claim 4.** Let  $D_{1,2,\dots,n}$  be  $n$  observations sampled from the distribution  $P_G$ . Let  $\hat{\beta}_n$  be the maximum likelihood estimate obtained by optimizing  $n^{-1} \sum_i \log P_F(D_i, \beta)$  where  $P_F(\cdot, \beta)$  is a parametric model. Then under certain assumptions

$$\sqrt{n}(\hat{\beta}_n - \beta^*) \xrightarrow{a.s.} \mathcal{N}(0, C(\beta^*)) \text{ as } n \rightarrow \infty$$

where  $\beta^*$  is the value of parameters which minimizes the KL divergence between the true and misspecified models and  $C$  is a covariance matrix functional dependent on  $P_F$  and  $P_G$ .

In the second stage estimation (Step 5 in Algorithm 1) we use maximum likelihood training to re-estimate the GLM models with  $\mathbb{E}[\mathcal{R}(Y_i)|\mathcal{R}(Y_{-i})]$  as a proxy for the noise variable. Hence the above result directly applies showing that our estimate of parameters is asymptotically normal.

To derive the relative efficiency of the SGLM approach vis a vis direct estimation, we need to compute the functional  $C$  using explicit formulas given in White (1994):

$$\begin{aligned} C &= A^{-1}(\theta^*)B(\theta^*)A^{-1}(\theta^*) \\ A &= \mathbb{E}_{P_G} \left[ \frac{\partial^2 \log P_F(Y|X, \theta^*)}{\partial \theta_i^* \partial \theta_j^*} \right] \\ B &= \mathbb{E}_{P_G} \left[ \frac{\partial \log P_F(Y|X, \theta^*)}{\partial \theta_i^*} \frac{\partial \log P_F(Y|X, \theta^*)}{\partial \theta_j^*} \right] \end{aligned}$$

where  $\mathbb{E}_{P_G}$  is expectation with respect to the true distribution  $P_G$ .

Let the covariates available in the fitted model be denoted as  $X_c$ . For the standard max likelihood estimation, the covariates  $X_c$  are  $X$ . On the other hand in SGLM we have an additional covariate obtained from the residuals. Note that for simplicity of exposition instead of explicitly writing this as an expectation like  $\mathbb{E}[\mathcal{R}(Y_1)|\mathcal{R}(Y_2)]$ , we abuse notation to denote the term by  $\mathcal{R}$ .

Then using the definition of canonical GLMs for the generative model in Figure 2(c) we get:

$$\begin{aligned} B &= \mathbb{E}_{X,N} [X_c^T X_c \mathbb{E}_{Y|X,N} [(Y - A'(\beta^* X_c))^2]] \\ &= \mathbb{E}_{X,N} [X_c^T X_c (\text{Var}(Y|X, N) + (\mathbb{E}[Y|X, N] - A'(\beta^* X_c))^2)] \\ A &= \mathbb{E}_{X,N} [X_c^T X_c \mathbb{E}_{Y|X,N} [-A''(\beta^* X_c)]] \end{aligned}$$

In the current generative model analysing the above expressions without further assumptions is intractable. Hence we limit to the the test for no effect of covariate factors i.e under the null hypothesis that  $Z_i$  being linearly independent of  $X$ . Under this hypothesis, both  $\mathbb{E}[Y|X, N]$  and  $\text{Var}[Y|X, N]$  becomes independent of covariates  $X$  and hence can be treated purely as a function of  $N$ . Secondly since the variance explicitly depends on the estimated  $\beta$  which again depends on the specific distribution of  $N, X$ , we make another assumption that the estimated  $\beta$  are the true values.

Under these assumptions, the terms including the log partition function  $A$  also become independent of  $X$ , allowing a factorization of the above expectations into product of expectations. Specifically we can factor out the  $X^T X$  terms (as  $X$  is independent of  $N$ ). Finally we also invoke the Claim 3 to argue that

$$N = \mathcal{R} + \epsilon_N$$

where  $\epsilon_N$  is unpredictable independent error of reconstructing  $N$ .

| GLM                                                             | SGLM                                                                          |
|-----------------------------------------------------------------|-------------------------------------------------------------------------------|
| $B = \mathbb{E}_N [(Var(Y N) + (A'(\beta_N N) - A'(0))^2)]$     | $B = \mathbb{E}_N [(Var(Y N) + (A'(\beta_N N) - A'(\beta_N \mathcal{R}))^2)]$ |
| $\approx \mathbb{E}_N [(Var(Y N)) + (\beta_N A''(0))^2 Var(N)]$ | $\approx \mathbb{E}_N [(Var(Y N)) + (\beta_N A''(0))^2 Var(\epsilon_N)]$      |

From the above expressions it is clear that the asymptotic relative variance of the estimator is determined by the strength of dependence on noise  $\beta_N$ , the inherent variability of  $Y$  and the reconstruction error of  $N$  from the residuals. When the reconstruction error is small (such as when the number of auxiliary variables is high) then SGLM can provide more powerful tests and better confidence intervals for parameter estimation. Similarly as one might expect if the conditional variance of  $Y$  is very high compared to the influence of  $N$  both methods have similar efficiency.

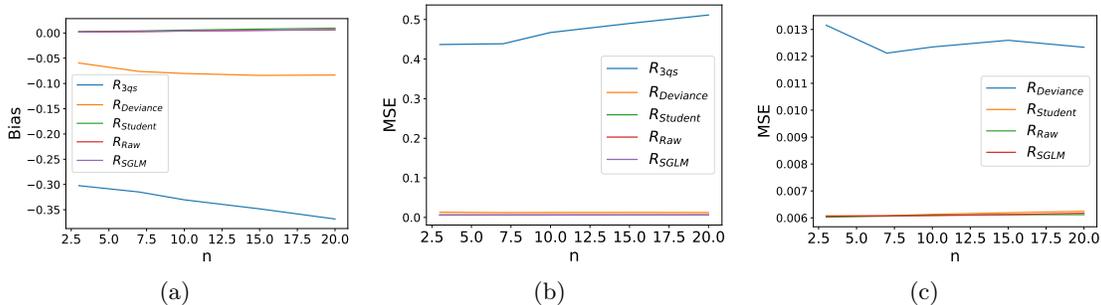

Figure 6: Results on synthetic data. Bias (a), and MSE for various Residual comparison (b,c) vs  $|Y_2|$  count  $n$  on Gamma regressions

## D Experimental Results: Gamma Regression

Figure 6 shows the estimation error for Gamma regression as a function of the dimension  $n$  of  $Y_{-1}$ , i.e., the number of auxiliary variables available for denoising. In Figure 6(a) we plot the bias against the true value of  $Z_1$  aggregated across the runs. In Figure 6(b,c) we have plotted the MSE of using different residuals and the method of Shankar et al. (2019)
